# Supplementary material for: Quantum-Classical Computing via Tensor Networks
Source: arXiv:2410.15080 source file (2024-10-19)
Supplement: Supplementary file 1 [file appendix.tex]

\section{Instantiations and Coefficient Tensors}

\subsection{Virtual CZ}

Instantiations

\begin{equation*}
    Inst_1 = Inst_2 = [S^{\dagger}, S, S^{\dagger} \circ Meas, I, Z]
\end{equation*}

\begin{equatio/n*}
    C_{\mathbf{CZ}} = \frac{1}{2} \begin{pmatrix}
        1 & 0 & 0 & 0 & 0 \\
        0 & 1 & 0 & 0 & 0 \\
        0 & 0 & 0 & 1 & -1 \\
        0 & 0 & 1 & 0 & 0 \\
        0 & 0 & -1 & 0 & 0 \\
    \end{pmatrix}
\end{equation*}

\subsection{Virtual RZZ}

Instantiations

\begin{equation*}
    Inst_1 = Inst_2 = [I, Z, Meas, S, S^{\dagger}]
\end{equation*}

\begin{equation*}
    C_{\mathbf{RZZ(\theta)}} = \frac{1}{2} \begin{pmatrix}
        cos(-\theta')^2 & 0 & 0 & 0 & 0 \\
        0 & sin(-\theta')^2 & 0 & 0 & 0 \\
        0 & 0 & 0 & -cs & cs \\
        0 & 0 & -cs & 0 & 0 \\
        0 & 0 & cs & 0 & 0 \\
    \end{pmatrix},
\end{equation*}
where 
\begin{equation*}
    \theta' = -\theta / 2,\ \text{and}\  cs = cos(\theta') \cdot sin(\theta')
\end{equation*}

\subsection{Virtual Wire}

To virtualize a wire, we need to first preprocess the results

After preprocessing, the coefficients of a virtual wire are

\begin{equation*}
    C_{\mathbf{Wire}} = \frac{1}{2} \circ I^{4\otimes 4}\ .
\end{equation*}

Preprocessing

\begin{equation*}
    C_{\mathbf{Wire}} = \frac{1}{2} \begin{pmatrix}
        & \ket{0} & \ket{1} & \ket{+} & \ket{i} \\
        I &  &  & & \\
        Z &  &  & & \\
        X &  &  & &  \\
        Y &  &  & & \\
        
    \end{pmatrix}
\end{equation*}
